# Supplementary material for: Global hybrid multiconfiguration pair-density functional theory
Source: arXiv:1911.11162 ancillary file (2019-11-25)
Supplement: Supplementary file 1 [file SuppInfo.pdf]

# Global hybrid multiconfiguration pair-density functional theory

Mohammad Mostafanejad,[†] Marcus Dante Liebenthal,[‡] and A. Eugene DePrince III[*,†]

† *Department of Chemistry and Biochemistry, Florida State University, Tallahassee, FL 32306-4390*

‡ *Department of Chemistry and Biochemistry, Ithaca College, Ithaca, NY 14850*

E-mail: deprince@chem.fsu.edu

# 1 The O3ADD6 set

In this section, we apply the multiconfiguration pair-density functional theory (MCPDFT) and multiconfiguration one-parameter hybrid pair-density functional theory ($\lambda$-MCPDFT) methods to the O3ADD6 data set, using the aug-cc-pVTZ basis set.[1] All molecular geometries were taken from Ref. 2. The relative energies of the stationary points and separated reactant molecules that comprise the O3ADD6 dataset are presented in Table S1.

Table S1: Calculated relative energies (kcal mol$^{-1}$) of the stationary points and separated reactant molecules that comprise the O3ADD6 dataset.

| Method | $N$-representability | $\lambda^a$ | $O_3 + C_2H_4 \rightarrow$ | | | $O_3 + C_2H_2 \rightarrow$ | | | MAE |
|---|---|---|---|---|---|---|---|---|---|
| | | | vdW | TS | Cycloadduct | vdW | TS | Cycloadduct | |
| tPBE | | 0.00 | -0.39 | 6.26 | -65.56 | -0.60 | 3.41 | -49.87 | 2.24 |
| tBLYP | DQG | 0.00 | 0.76 | 10.37 | -57.21 | 0.60 | 6.82 | -42.18 | 5.47 |
| tSVWN3 | | 0.00 | -2.43 | -5.24 | -83.93 | -3.65 | -7.08 | -67.94 | 9.43 |
| $\lambda$-tPBE | | 0.20 | -0.42 | 7.84 | -67.75 | -2.19 | 4.91 | -57.66 | 1.30 |
| $\lambda$-tBLYP | DQG | 0.35 | 0.24 | 12.51 | -61.41 | -2.70 | 8.82 | -56.18 | 2.75 |
| $\lambda$-tSVWN3 | | 0.50 | -1.15 | 7.72 | -73.88 | -5.72 | 4.69 | -72.34 | 5.19 |
| ftPBE | | 0.00 | -0.42 | 7.78 | -68.71 | 1.09 | 5.21 | -49.84 | 3.10 |
| ftBLYP | DQG | 0.00 | 0.72 | 11.28 | -60.75 | 1.62 | 7.85 | -42.89 | 5.25 |
| ftSVWN3 | | 0.00 | -2.44 | -5.09 | -87.58 | -3.18 | -6.88 | -68.70 | 10.03 |
| $\lambda$-ftPBE | | 0.20 | -0.44 | 9.07 | -70.17 | -0.82 | 6.37 | -57.59 | 2.28 |
| $\lambda$-ftBLYP | DQG | 0.35 | 0.20 | 12.98 | -63.64 | -2.19 | 9.33 | -56.73 | 2.35 |
| $\lambda$-ftSVWN3 | | 0.50 | -1.16 | 7.85 | -75.48 | -5.45 | 4.84 | -72.60 | 5.49 |
| tPBE | | 0.00 | -0.39 | 5.50 | -66.04 | -0.85 | 2.78 | -50.05 | 2.46 |
| tBLYP | DQG+T2 | 0.00 | 0.77 | 9.60 | -57.71 | 0.32 | 6.17 | -42.39 | 5.07 |
| tSVWN3 | | 0.00 | -2.42 | -6.04 | -84.44 | -3.91 | -7.75 | -68.15 | 9.84 |
| $\lambda$-tPBE | | 0.20 | -0.40 | 7.69 | -68.00 | -1.86 | 4.87 | -57.57 | 1.29 |
| $\lambda$-tBLYP | DQG+T2 | 0.35 | 0.27 | 12.82 | -61.51 | -1.97 | 9.23 | -55.88 | 2.78 |
| $\lambda$-tSVWN3 | | 0.45 | -1.26 | 6.92 | -75.19 | -4.51 | 4.10 | -71.78 | 5.13 |
| ftPBE | | 0.00 | -0.41 | 7.03 | -68.98 | 0.75 | 4.57 | -49.97 | 3.08 |
| ftBLYP | DQG+T2 | 0.00 | 0.73 | 10.51 | -61.06 | 1.27 | 7.18 | -43.05 | 4.88 |
| ftSVWN3 | | 0.00 | -2.43 | -6.06 | -88.13 | -3.55 | -7.71 | -69.04 | 10.54 |
| $\lambda$-ftPBE | | 0.20 | -0.42 | 8.94 | -70.26 | -0.56 | 6.33 | -57.45 | 2.29 |
| $\lambda$-ftBLYP | DQG+T2 | 0.35 | 0.24 | 13.30 | -63.62 | -1.50 | 9.73 | -56.40 | 2.57 |
| $\lambda$-ftSVWN3 | | 0.45 | -1.26 | 6.97 | -77.00 | -4.27 | 4.19 | -72.15 | 5.46 |
| Reference values$^b$ | | — | -1.90 | 7.74 | -63.80 | -1.94 | 3.37 | -57.15 | — |

[a] The optimal mixing parameter.
[b] Best estimates from Ref. 2.

# 2 Non-parallelity errors in $H_2O$ molecule

Figure S1 details the effect of the mixing parameter, $\lambda$, on the NPE for $H_2O$ molecule. Specifically, when enforcing the PQG (PQG+T2) $N$-representability conditions and adopting tSVWN3, tPBE, tBLYP, ftSVWN3, ftPBE, and ftBLYP functionals, the optimal $\lambda$ values are 0.70 (0.70), 0.45 (0.50), 0.45 (0.50), 0.70 (0.70), 0.50 (0.50), and 0.50 (0.50), respectively.

Figure S1: The NPE in the dissociation curves for the $H_2O$ molecule as a function of the mixing parameter, $\lambda$, when using PQG (a),(b) and PQG+T2 (c),(d) $N$-representability conditions and translated (a),(c) or fully-translated (b),(d) $\lambda$-MCPDFT functionals.

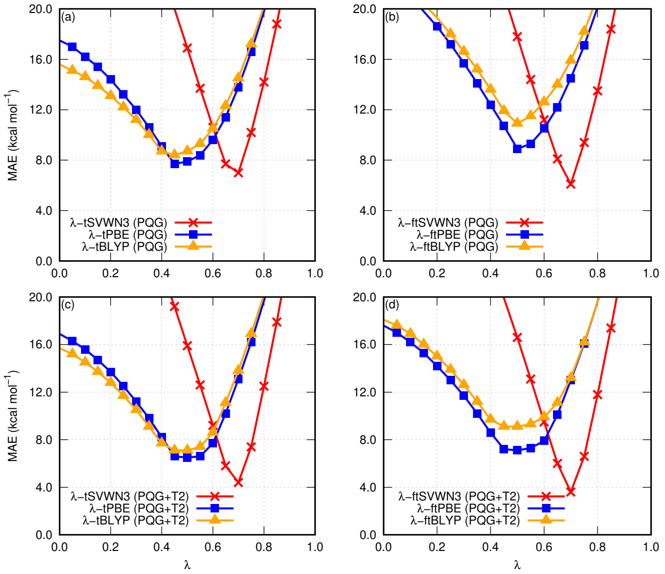

# 3 Potential Energy Curves of $N_2$ and $H_2O$ molecules

## References


(1) Dunning, T. H. Gaussian basis sets for use in correlated molecular calculations. I. The atoms boron through neon and hydrogen. *J. Chem. Phys.* **1989**, *90*, 1007–1023.

(2) Zhao, Y.; Tishchenko, O.; Gour, J. R.; Li, W.; Lutz, J. J.; Piecuch, P.; Truhlar, D. G. Thermochemical Kinetics for Multireference Systems: Addition Reactions of Ozone. *J. Phys. Chem. A* **2009**, *113*, 5786–5799.
